# Supplementary material for: Impact of the reference choice on scalp EEG connectivity estimation
Source: arXiv:1812.00794 source file (2019-01-24)
Supplement: Supplementary file 1 [file supplementary_material.pdf]

**Supplementary Material**

Chella, F., Pizzella, V., Zappasodi, F., Marzetti, L. (2016). Impact of the reference choice on scalp EEG connectivity estimation. *Journal of Neural Engineering*, 13, 036016. DOI: https://doi.org/10.1088/1741-2560/13/3/036016

## *S.1. Effects of ESD discretization on REST performance*

*S.1.1. Rationale and simulation settings.* An appealing feature of REST is that, to perform data re-referencing at infinity, it is not strictly required to know the actual neuronal sources generating the EEG potentials, but it is sufficient to assume an equivalent source distribution (ESD), where the equivalence means that the ESD generates the same potentials of the actual sources. To this purpose, three different ESD models were proposed in literature, including a dipole layer (Sidman et al. 1992), a charge layer (Yao 1996) and a multipole series at the origin of the coordinate system (Yao 2000). All these models are consistent to each other, namely the other two can be deduced when one is known (Yao 2000).

In the present study, the dipole layer was chosen as ESD for its simplicity in realization and relative better performance (Yao 2001), as done previously in literature (e.g. Marzetti et al. 2007, Yao 2001, Yao et al. 2005). In theory, the equivalent dipole layer should be a continuous and closed layer of current dipoles enclosing all the possible neuronal sources. In practice, since computers only allow a discrete representation of the closed surface, the REST transformed potentials will be affected by an approximation error, which depends on the degree of discretization applied to the surface. Thus, it is important to study this effect by using simulations.

In general, a larger number of evenly spaced dipoles results in a better approximation of the continuous layer, but at the expense of higher computational efforts. With the present implementation of REST, the computational efforts for a desktop PC (Intel® i5 - 2400 CPU @ 3.10 GHz; RAM 8 GB) become excessive when the number of dipoles exceeds 4000. Based on this limit, we investigated whether the number of dipoles ranging from a few hundreds (with relatively low computational efforts) to a few thousands (with relatively high computational efforts) has a crucial impact on the performances of REST. To this aim, we performed a simulation study where the generation of simulated data follows the same pipeline described in section 2.3 of the paper, that is, 1000 datasets were generated from randomized source configurations, and for different electrode densities (i.e. 21, 34, 74 or 128 electrodes). We then focused only the re-referencing using REST for different head models (i.e. *spherical*, *standard*, *real perturbed* or *real exact* head model). Additionally, and of specific interest to this study, simulations were repeated for different numbers of current dipoles forming the ESD, which were assumed to be 400, 1000 or 4000. No noise was added to the data, in order to exclude any confound from the analysis of the effects of the ESD discretization. The effectiveness of the REST was evaluated on the basis of the relative errors ($RE$) for potentials and for the imaginary part of coherency, as defined in equations (14) and (15) of the paper. Statistical analysis for the contrast of $RE$ distributions for different numbers of dipoles forming the ESD consisted of non-parametric independent sample statistics, i.e. Wilcoxon-Mann-Whitney test.

*S.1.2. Simulation results.* Figure S.1 shows the mean values of the relative error ($RE$) for potentials (on the left panel) and for the imaginary part of coherency (on the right panel), for all the combinations of the following parameters: number of EEG electrodes, head model used for REST re-referencing, and number of current dipoles forming the ESD. We can observe that, apart from an overall decrease of $RE$ for

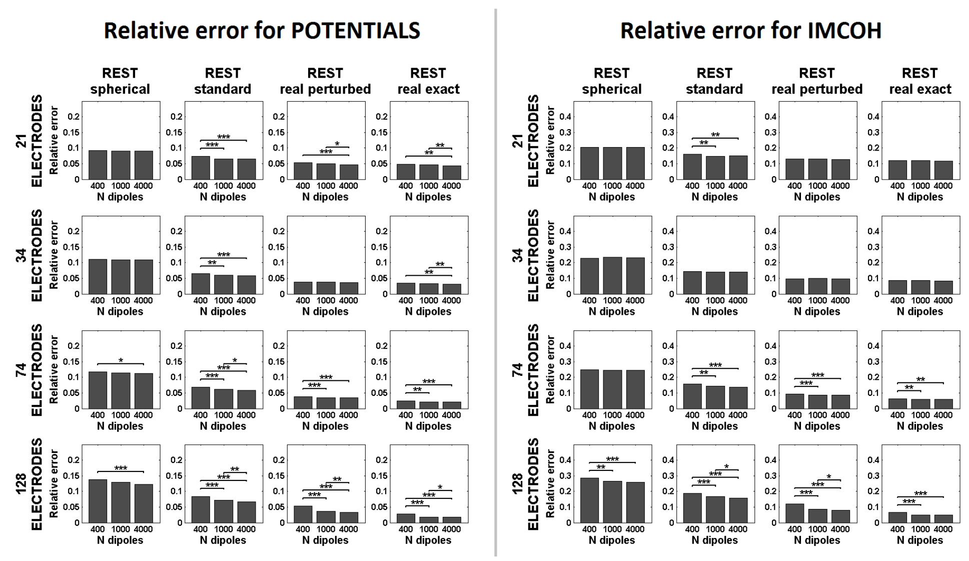


**Figure S.1.** Effects of ESD discretization on REST performance. Figure shows the mean values of the relative error ($RE$) for potentials (on the left panel) and for the imaginary part of coherency (on the right panel), for all the combinations of the following parameters: number of EEG electrodes, head model used for REST re-referencing, and number of current dipoles forming the ESD. The $p$-values resulting from the non-parametric Wilcoxon-Mann-Whitney test, performed to contrast the distributions of $RE$s obtained from all simulation repetitions, have been denoted by $*$ ($p < 0.05$), $**$ ($p < 0.01$) and $***$ ($p < 0.001$).

increasing head model accuracy and increasing electrode density, which was already discussed in sections 3.1.1 and 3.1.2, the number of dipoles has a non-negligible effect on the performances of REST, with a larger number of dipoles resulting in a smaller $RE$. Statistical analysis revealed that observed differences for $RE$ are significant when the performances of REST improve due to enhanced head model accuracy or enhanced electrode density, i.e. at various level of statistical significance as indicated by the p-values given in figure S.1. Based on the above results, we can conclude that 4000 dipoles is the proper number of dipoles to perform REST re-referencing.

Nevertheless, it is important to note that, although the REST performances have been shown to decrease when the ESD consists of only 400 current dipoles, REST still outperforms all the other references concerned in this paper. This can be seen in figure S.2, where, in analogy with the results shown in figures **??** and 4 of the paper, we show the results for $RE$ for potentials (panel a) and for the imaginary part of coherency (panel b), but with the difference that now REST is performed by assuming an ESD consisting of only 400 current dipoles. These results show that the relative error

obtained with REST is always smaller ($p < 0.001$) than the $RE$ obtained with other references, i.e. Cz, DLM and AVE, thus demonstrating the superior performance of re-referencing using REST.

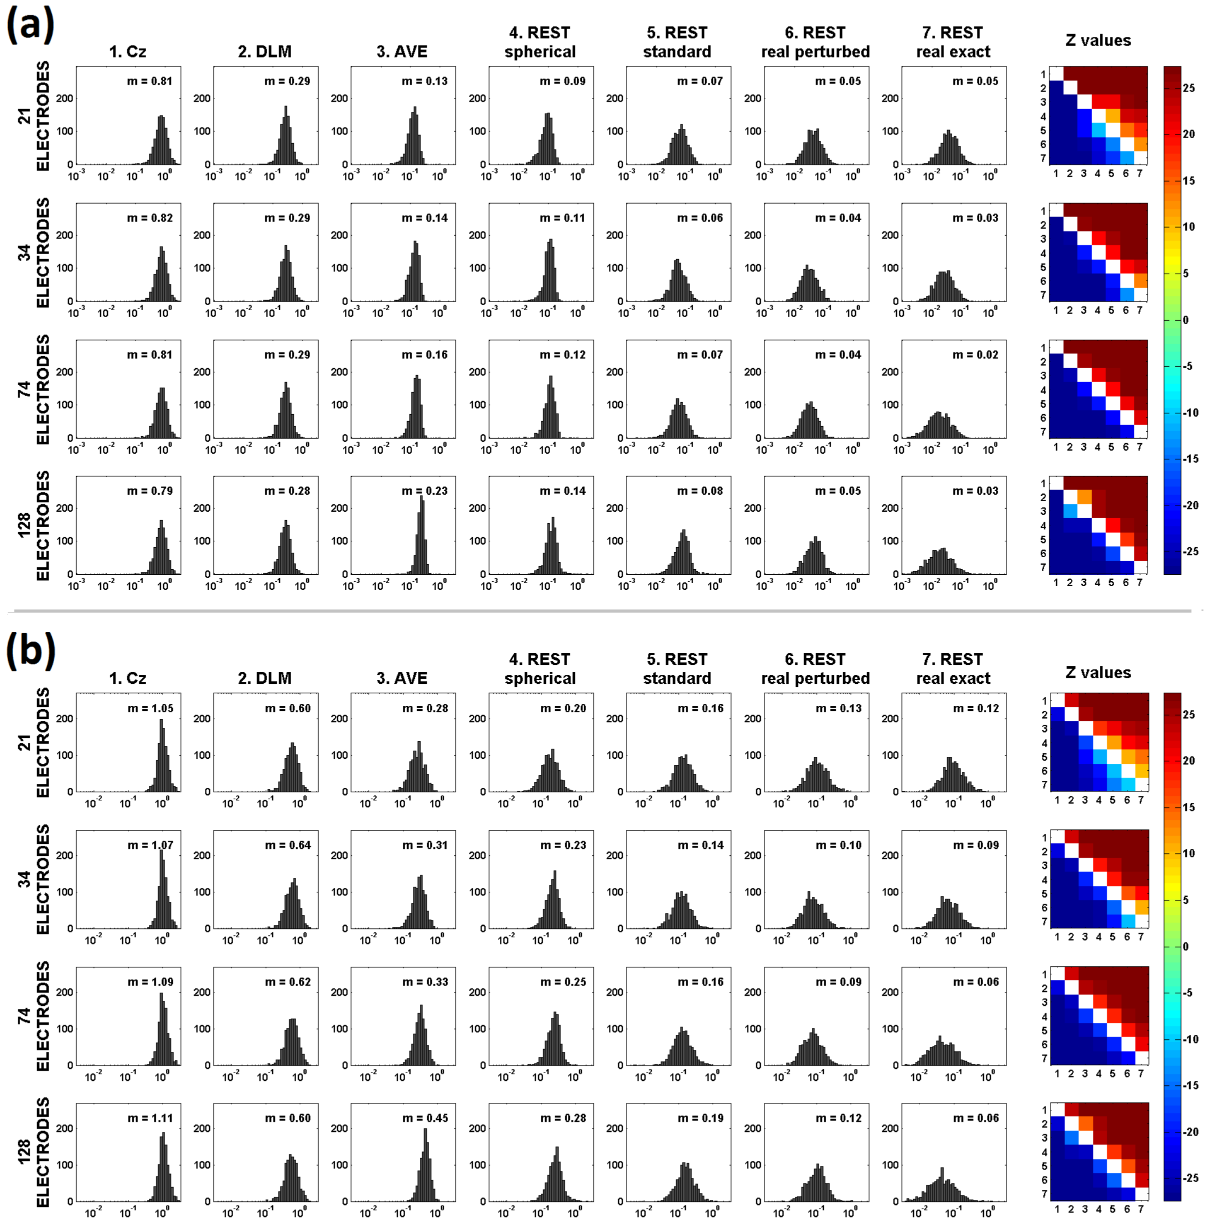


**Figure S.2.** Effects of ESD discretization on REST performance. Histograms of the relative error ($RE$) for potentials (panel a) and for the imaginary part of coherency (panel b), i.e. for all combinations of number of EEG electrodes and EEG referencing conditions, when REST is performed by assuming an ESD consisting of 400 current dipoles randomly located and normally oriented on the cortical surface. The histograms collect the data from 1000 simulation repetitions. The mean value for $RE$ is denoted by $m$. For the ease of visualization, the abscissa values for the histograms have been scaled logarithmically. Simulated EEG data were not corrupted by noise. Rightmost side of each panel: z-values for non-parametric paired sample statistics, i.e. Wilcoxon signed-rank test, performed for the contrast of the $RE$ distributions obtained in different EEG referencing conditions, here labelled with a progressive number from 1 to 7, and for a specific electrode density.

*S.2. Supplementary figure to section 2.3.3*

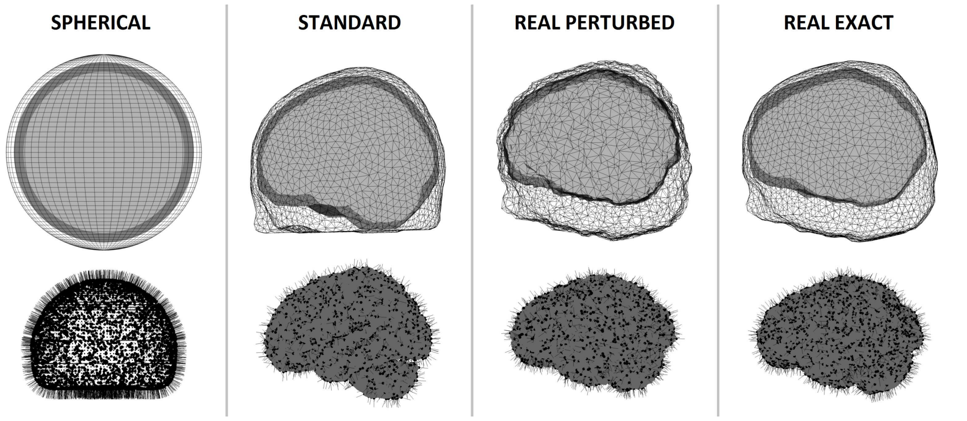


**Figure S.3.** Head models used for the computation of the REST transformation matrix. On the top row, the three shell volume conductor models. On the bottom row, the equivalent source distribution (ESD) consisting of 4000 current dipoles randomly located over a spherical cap (for the spherical model) or over the cortical mantle (for other models).

*S.3. Supplementary figure to section 3.1.2*

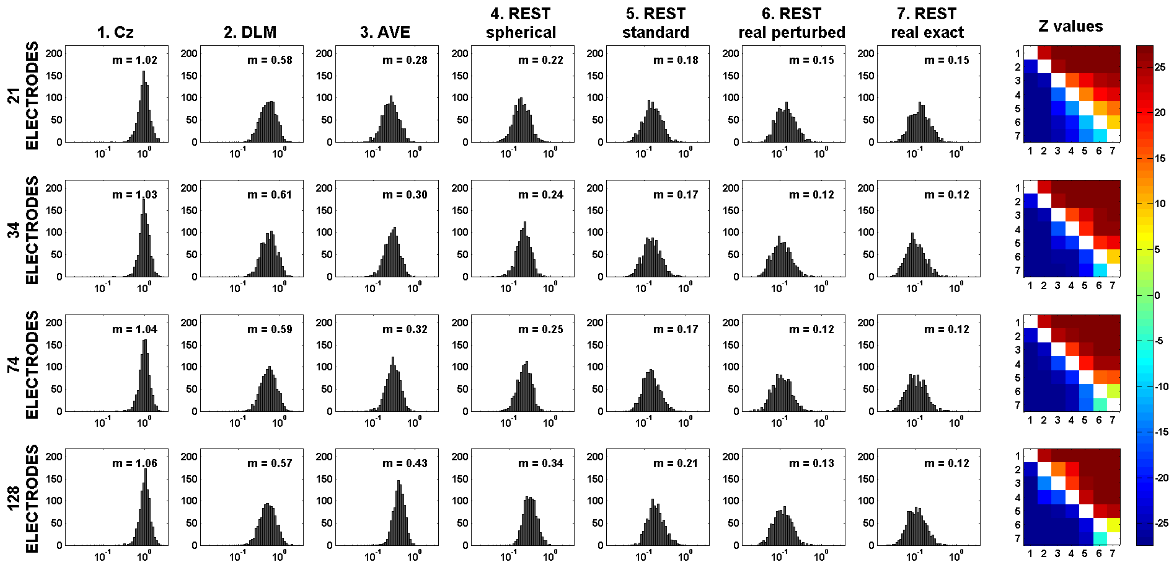


**Figure S.4.** Histograms of the relative error ($RE$) for the imaginary part of coherency estimated from the EEG recordings with additive iso-spectral instrumentation noise (SNR=10). The histograms are shown for all combinations of number of EEG electrodes and EEG referencing conditions, and collect the data from 1000 simulation repetitions. The mean value for $RE$ is denoted by $m$. For the ease of visualization, the abscissa values for the histograms have been scaled logarithmically. In the rightmost side of the panel (b): z-values (all significant at the $p < 0.001$ level) for non-parametric paired sample statistics, i.e Wilcoxon signed-rank test, performed for the contrast of the $RE$ distributions obtained in different EEG referencing conditions, here labelled with a progressive number from 1 to 7, and for a specific electrode density.

*S.4. Supplementary figure to section 3.2.1*

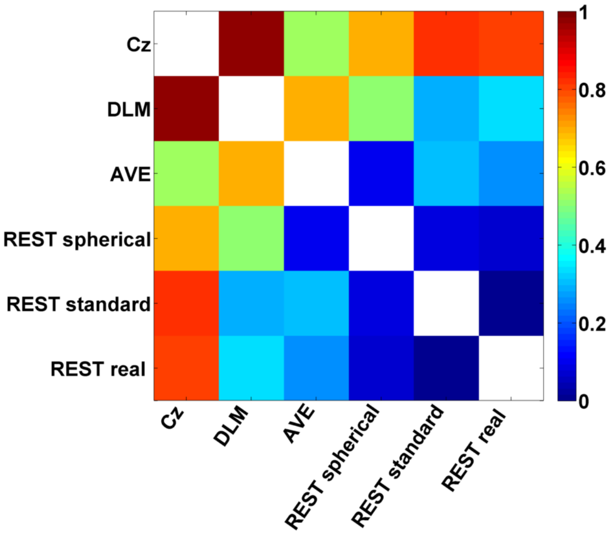


**Figure S.5.** Comparison between the all-to-all connectomes based on the imaginary part of coherency obtained for different EEG references used in the representation of real EEG data. The matrix shows the dissimilarity measures defined as one minus the squared Pearson correlation coefficient, i.e. $d = 1 - r^2$, between vector-like data obtained by unfolding the imaginary part of coherency matrices.

## References

Marzetti, L., Nolte, G., Perrucci, M. G., Romani, G. L. & Del Gratta, C. (2007). The use of standardized infinity reference in EEG coherency studies, *NeuroImage* **36**(1): 48 – 63.

Sidman, R. D., Vincent, D. J., Smith, D. B. & Lee, L. (1992). Experimental tests of the cortical imaging technique-applications to the response to median nerve stimulation and the localization of epileptiform discharges, *Biomedical Engineering, IEEE Transactions on* **39**(5): 437–444.

Yao, D. (1996). The equivalent source technique and cortical imaging, *Electroencephalography and Clinical Neurophysiology* **98**(6): 478 – 483.

Yao, D. (2000). High-resolution EEG mappings: a spherical harmonic spectra theory and simulation results, *Clinical Neurophysiology* **111**(1): 81 – 92.

Yao, D. (2001). A method to standardize a reference of scalp eeg recordings to a point at infinity, *Physiological Measurement* **22**(4): 693.

Yao, D., Wang, L., Oostenveld, R., Nielsen, K. D., Arendt-Nielsen, L. & Chen, A. C. N. (2005). A comparative study of different references for eeg spectral mapping: the issue of the neutral reference and the use of the infinity reference, *Physiological Measurement* **26**(3): 173.
